# Supplementary material for: On the Transferability of Minimal Prediction Preserving Inputs in Question Answering
Source: arXiv:2009.08070 source file (2021-03-25)
Supplement: Supplementary file 1 [file mppi_appendices.tex]

% \documentclass[11pt,a4paper]{article}
% \usepackage[hyperref]{naacl2021}
% \usepackage{times}
% \usepackage{latexsym}
% \usepackage{amsfonts}
% \renewcommand{\UrlFont}{\ttfamily\small}

% % This is not strictly necessary, and may be commented out,
% % but it will improve the layout of the manuscript,
% % and will typically save some space.
% \usepackage{microtype}
% \usepackage{float}
% \usepackage{amsmath}
% \usepackage{appendix}
% \usepackage{float}
% \usepackage{textcomp}
% % \usepackage[disable]{todonotes}
% \usepackage{booktabs}

% \usepackage{todonotes}
% \usepackage{booktabs}

% %\aclfinalcopy % Uncomment this line for the final submission
% %\def\aclpaperid{***} %  Enter the acl Paper ID here

% %\setlength\titlebox{5cm}
% % You can expand the titlebox if you need extra space
% % to show all the authors. Please do not make the titlebox
% % smaller than 5cm (the original size); we will check this
% % in the camera-ready version and ask you to change it back.

% \newcommand\BibTeX{B\textsc{ib}\TeX}
% \newcommand{\squad}{\textsc{SQuAD}}
% \newcommand{\snli}{\textsc{SNLI}}
% \newcommand{\mnli}{\textsc{MNLI}}
% \newcommand{\vqa}{\textsc{VQA}}
% \newcommand{\nlp}{\textsc{NLP}}
% \newcommand{\mppi}{\textsc{MPPI}}
% \newcommand{\qa}{\textsc{QA}}
% \newcommand{\lstm}{\textsc{LSTM}}
% \newcommand{\drqa}{\textsc{DrQA}}
% \newcommand{\bert}{\textsc{Bert}}
% \newcommand{\xlnet}{\textsc{XLNet}}
% \newcommand{\abr}[1]{\textsc{#1}}
% \newcommand{\respace}{\vspace*{-.1cm}}

% \definecolor{coloranswer}{HTML}{0596FF}
% \newcommand*{\mybox}[2]{\tikz[anchor=base,baseline=0pt,rounded corners=0pt, inner sep=0.2mm] \node[fill=#1!60!white] (X) {#2};}

% \begin{document}
% 	\appendix
% 	\appendixpage
	
% 	\label{sec:appendix}
	
% 	\section{Reproducibility}
% 	\subsection{Question Answering Models}
% 	For reproducibility, we share our hyper-parameter selection in Table~\ref{appendix-hyperparams}. 
% 	We borrow our hyper-parameters from \citet{longpre2019exploration} for training all Question Answering (QA) models. 
% 	Their parameters are tuned for the same datasets in the MRQA Shared Task. 
% 	We found these choices to provide stable and strong results across all datasets.
	
% 	Our BERT and XLNet question answering modules build upon the standard PyTorch \citep{NEURIPS2019_9015} implementations from HuggingFace, and are trained on $8$ NVIDIA Tesla V100 GPUs.\footnote{\url{https://github.com/huggingface/transformers}}
% 	For \abr{DrQA}, by \citet{chen2017reading}, we borrowed the implementation and hyper-parameters from hitvoice (\url{https://github.com/hitvoice/DrQA}) and train on $1$ NVIDIA Tesla V100 GPU.\footnote{We used the open source version available at \url{https://github.com/hitvoice/drqa}.} 
	
% 	\begin{table}[htb]
% 		\small
% 		\centering
% 		\begin{tabular}{ll}
% 			\toprule
% 			\textbf{Model Parameter} & \textbf{Value} \\
% 			\midrule
% 			\textbf{\abr{DrQA}} & {} \\
% 			\midrule
% 			Model Size (\# params) & $31.5M$ \\
% 			Avg. Train Time & $10h\ 30m$ \\
% 			\midrule
% 			Learning Rate & 0.1 \\
% 			Optimizer & Adamax \\
% 			Num Epochs & 35 \\
% 			Batch size & 32 \\
% 			Dropout & 0.4 \\
% 			Hidden size & 128 \\
% 			\midrule
% 			\textbf{BERT-BASE} & {} \\
% 			\midrule
% 			Model Size (\# params) & $108.3M$ \\
% 			Avg. Train Time & $2h\ 20m$ \\
% 			\midrule
% 			Learning Rate & $5e-5$ \\
% 			Optimizer & Adam \\
% 			Num Epochs & 2 \\
% 			Batch Size & 25 \\
% 			Gradient Accumulation & 1 \\
% 			Dropout & $0.1$ \\
% 			Lower Case & False \\
% 			Max Query Length & 64 \\
% 			Max Sequence Length & 512 \\
% 			\midrule
% 			\textbf{XLNet-LARGE} & {} \\
% 			\midrule
% 			Model Size (\# params) & $364.5M$ \\
% 			Avg. Train Time & $4h\ 45m$ \\
% 			\midrule
% 			Learning Rate & $2e-5$ \\
% 			Optimizer & Adam \\
% 			Num Epochs & 2 \\
% 			Batch Size & 6 \\
% 			Gradient Accumulation & 3 \\
% 			Dropout & $0.1$ \\
% 			Lower Case & False \\
% 			Max Query Length & 64 \\
% 			Max Sequence Length & 512 \\
% 			\bottomrule
% 		\end{tabular}
% 		\caption{\label{appendix-hyperparams}
% 			Hyperparameter selection for each model type.
% 		}
% 	\vspace*{-.5cm}
% 	\end{table}
	
% 	\subsection{Dataset}
	
% 	We employ 6 diverse QA training sets and 12 evaluation sets from the MRQA 2019 workshop (\url{https://github.com/mrqa/MRQA-Shared-Task-2019}) \citep{fisch2019mrqa}. 
% 	These datasets have been normalized into purely extractive format and all questions are answerable. 
% 	The 6 training datasets are SQuAD \citep{rajpurkar2016squad}, NewsQA \citep{trischler2016newsqa}, TriviaQA \citep{joshi2017triviaqa}, SearchQA \citep{dunn2017searchqa}, HotpotQA \citep{yang2018hotpotqa}, and Natural Questions \citep{kwiatkowski2019natural}. 
% 	Six other evaluation datasets are included: BioASQ \citep{tsatsaronis2012bioasq}, DROP \citep{dua2019drop}, DuoRC \citep{saha2018duorc}, RACE \citep{lai2017race}, RelationsExtraction \citep{levy2017zero} , and TextbookQA \citep{kembhavi2017you}. 
% 	Table~\ref{dataset-stat} shows their statistics.
	
% 	\begin{table*}
%     \footnotesize
%     \centering
%     \tabcolsep=0.25cm
%     \begin{tabular}{lllrrrr@{}}
%     \textbf{Dataset}                               & \textbf{Question (Q)} & \textbf{Context (C)} & \textbf{{Avg. Q Len}} & \textbf{Avg. C Len}  & \textbf{Train} & \textbf{Dev} \\ 
%     \toprule
%     SQuAD & Crowdsourced      & Wikipedia  & 11  &  137  & 86,588         & 10,507       \\
%     NewsQA & Crowdsourced      & News articles    & 8 & 599  & 74,160         & 4,212        \\
%     TriviaQA & Trivia            & Web snippets   & 16 & 784 & 61,688         & 7,785        \\
%     SearchQA & Jeopardy          & Web snippets & 17 & 749 & 117,384        & 16,980       \\
%     HotpotQA & Crowdsourced      & Wikipedia    &  22 & 232 & 72,928         & 5,904\\
%     Natural Questions & Search logs       & Wikipedia     & 9  & 153 & 104,071        & 12,836\\ 
%     \midrule
%     BioASQ & Domain experts    & Science articles & 11 & 248  & -              & 1,504 \\
%     DROP & Crowdsourced      & Wikipedia &   11  &  243  & -              & 1,503 \\
%     DuoRC & Crowdsourced      & Movie plots   & 9 & 681 & -              & 1,501\\
%     RACE & Domain experts          & Examinations   & 12 & 349 & -              & 674          \\
%     RelationExtraction   & Synthetic         & Wikipedia    & 9 &  30  & -              & 2,948      \\
%     TextbookQA & Domain experts    & Textbook & 11   &   657  & - & 1,503\\ 
%     \bottomrule
%     \end{tabular}
%     \caption{Statistics about datasets used: The first block presents six domains used for training, the second block presents six additional domains used for model evaluation and generating \mppi{}s.}
%     \label{dataset-stat}
%     \vspace*{-.2cm}
%     \end{table*}
    
%     We use the hyperparameters described in Table~\ref{appendix-hyperparams} for training on each dataset.
%     We use all the training data provided for each by \textsc{MRQA}.
	
% 	\subsection{Generating \mppi{}s}
	
% 	The process for generating \mppi{}s closely follows the procedure described by \citet{feng2018pathologies}. 
% 	We operate with a beam size of $k=3$, finding that larger beam sizes exhibit diminishing returns, and rarely produce different results. 
% 	The procedure involves iteratively removing the token which is ``least important" to the model.
% 	The least important token is defined as the one that when removed provides the smallest decrease in confidence in the originally predicted span.
% 	Note that in some cases confidence in the originally predicted span can even increase with the removal of a token.
% 	In any case, the least important token is always designated by the lowest confidence in the original prediction.
% 	The stop condition is when removing \textbf{any} additional token would change the model's prediction. 
	
% 	Note that we follow previous work in only removing words from the query in extractive question answering. 
% 	The reason for this is the \mppi{} can be poorly defined when context tokens are removed.
% 	Since the output predictions are over the context tokens for extractive question answering, its possible to warp the answer space, or remove the answer altogether.
% 	Additionally, if we do not permit any alterations to the original prediction tokens, then there exists a trivial solution: remove all tokens except for the predicted answer.
% 	In this case an extractive question answering model is forced to predict that answer, with no alternative options.
% 	Consequently, \mppi{}s that allow modifications to the context, or output space, can be poorly defined.
% 	Since in question answering the query is an essential input to provide confident answers, we believe this is the most reasonable setup for the task.
	
% 	\begin{equation}\label{eq:1}
% 	p_{ij} = \max(\text{softmax}(S_i + E_j))
% 	\end{equation}
	
% 	For completeness, we describe our method of computing span confidence for question answering, given that there are many variations. 
% 	Let $S \in \mathbb{R}^{N}$ be the vector of start logits and $E \in \mathbb{R}^{N}$ be the vector of end logits, both of sequence length $N$. 
% 	For every combination of $i,\ j \in [0,N]$ where $j \ge i \le min(j+C,\ N)$, and $C=30$ is the maximum answer span length, we compute the confidence for that span of answer text as the sum of their respective logits $S_i + E_j$. 
% 	The final confidence probability $p_ij$ for a given span is as shown in Equation~\ref{eq:1}.
	
% 	The model, on the other hand, can still make the same prediction as it did on the full input, and with a similar degree of confidence. 
	
% 	\subsection{Regularizing \mppi{}s}
	
	
% 	There are a couple differences between the \mppi{} entropy-regularization strategy employed in this work and in \citet{feng2018pathologies}. 
% 	While \citet{feng2018pathologies} fine-tune an a model already trained for the question answering task, we regularize \mppi{}s in the initial fine-tuning stage (starting from BERT and XLNet's pre-trained weights). 
% 	Secondly, they alternate updates between two optimizers, one batch of maximum likelihood, two for \mppi{} entropy maximization, whereas we use the same optimizer and shuffle together equal numbers of \mppi{} and regular inputs. 
% 	We find our method (without rigorous comparison) to be slightly more effective on BERT at mitigating the \mppi{} phenomenon (measured by subsequent \mppi{} length). 
% 	We suspect, if there is an advantage, it is due to the regularization beginning with the start of fine-tuning, rather than on a subsequent stage of fine-tuning.
	
% 	\begin{equation} \label{eq:reg-ent}
% 	\mathcal{L_{MPPI}}=C-\lambda\sum_{\tilde{x}\in \tilde{\mathcal{X}}}
% 	\mathbb{H}\left(f(y | \tilde{x})\right)
% 	\end{equation}
	
% 	\begin{equation} \label{eq:final-loss}
% 	\mathcal{L}=\mathcal{L_{QA}}+\mathcal{L_{MPPI}}
% 	\end{equation}
	
% 	For completeness, we provide our entropy regularization loss term in Equation~\ref{eq:reg-ent}. 
% 	Let $\tilde{\mathcal{X}}$ denote the set of inputs that have been reduced to their \mppi{}, $\mathbb{H}\left(\cdot\right)$ denote the entropy and $f(y | x)$ denote the predicted confidence for $y$ given $x$. 
% 	We then represent the loss term for \mppi{}s as $\mathcal{L_{MPPI}}$, where the constant $C=10$ is chosen such that maximizing the entropy will minimize the loss. 
% 	We use $\lambda=0.1$ as the most effective choice in our limited set of trials. 
% 	The full loss term, for all inter-mixed regular question answering, and \mppi{} examples is the sum of standard QA loss $\mathcal{L_{QA}}$, and the \mppi{} loss term $\mathcal{L_{MPPI}}$, as shown in Equation~\ref{eq:final-loss}.
	
% 	In Figure~\ref{fig:reg-vs-pathos-f1-appendix} we display the full comparison between the performances of the \mppi{} regularized models and the regular models on 13 QA datasets, including Adversarial SQuAD \citep{jia2017adversarial}.
	
%     \begin{figure*}
% 		\centering
% 		\includegraphics[width=\linewidth]{figures/reg-vs-pathos-f1-v3.pdf}
% 		\caption{The generalization and robustness of \abr{BERT} models evaluated on 12 datasets, as well as Adversarial SQuAD. The ``(*)" indicates \mppi{}-regularization during training.}
% 		\label{fig:reg-vs-pathos-f1-appendix}
% 		\vspace*{-.4cm}
% 	  \end{figure*}
	
% 	\section{How do \mppi{} Lengths Compare?}
	
% 	In the main paper we describe the differences in length distributions between original and \mppi{} queries.
% 	To provide more detail into the length distributions we plot histograms of the query word lengths, for the original queries, \mppi{} queries, and \mppi{} queries after the \mppi{} regularization procedure.
% 	These lengths are plotted below for SQuAD (Figure~\ref{fig:squad-lens}), HotpotQA (Figure~\ref{fig:hotpot-lens}), NewsQA (Figure~\ref{fig:news-lens}), Natural Questions (Figure~\ref{fig:nq-lens}), TriviaQA (Figure~\ref{fig:trivia-lens}), and SearchQA (Figure~\ref{fig:search-lens}).
	
% 	\begin{figure}[H]
% 		\includegraphics[width=1\linewidth]{figures/squad_question_len.pdf}
% 		\caption{\abr{SQuAD} question length generated by different \mppi{} reduction methods}
% 		\label{fig:squad-lens}
% 		\vspace*{-.4cm}
% 	\end{figure}
% 	\begin{figure}[H]
% 		\includegraphics[width=1\linewidth]{figures/hotpot_question_len.pdf}
% 		\caption{\abr{HotpotQA} question length generated by different \mppi{} reduction methods}
% 		\label{fig:hotpot-lens}
% 		\vspace*{-.4cm}
% 	\end{figure}
	
% 	\begin{figure}[H]
% 		\includegraphics[width=1\linewidth]{figures/newsqa_question_len.pdf}
% 		\caption{\abr{NewsQA} question length generated by different \mppi{} reduction methods}
% 		\label{fig:news-lens}
% 		\vspace*{-.4cm}
% 	\end{figure}
	
% 	\begin{figure}[H]
% 		\includegraphics[width=1\linewidth]{figures/nq_question_len.pdf}
% 		\caption{\abr{NatrualQuestion} question length generated by different \mppi{} reduction methods}
% 		\label{fig:nq-lens}
% 		\vspace*{-.4cm}
% 	\end{figure}
	
% 	\begin{figure}[H]
% 		\includegraphics[width=1\linewidth]{figures/triviaqa_question_len.pdf}
% 		\caption{\abr{TriviaQA} question length generated by different \mppi{} reduction methods}
% 		\label{fig:trivia-lens}
% 		\vspace*{-.4cm}
% 	\end{figure}
	
% 	\begin{figure}[H]
% 		\includegraphics[width=1\linewidth]{figures/searchqa_question_len.pdf}
% 		\caption{\abr{SearchQA} question length generated by different \mppi{} reduction methods}
% 		\label{fig:search-lens}
% 		\vspace*{-.4cm}
% 	\end{figure}
	
% 	The query length distributions show that \mppi{}s are significantly shorter than original queries, with the \mppi{}s of regularized models somewhere in between.
% 	These length distributions may be sufficient to explain why humans find the non-regularized \mppi{}s completely uninterpretable, and the regularized \mppi{}s somewhat more interpretable.
	
% % 	\section{Are \mppi{}s Human Insufficient?}
	
% % 	In the main paper we define the ``human insufficiency" property as the inability for humans to make accurate or confident predictions on most \mppi{}s.
% % 	This can be roughly measured in F1 or Exact Match --- the human performance on the question answering task, using \mppi{} queries. 
% % 	\citet{feng2018pathologies} began benchmarking this measure of human interpretability with \abr{DrQA} on \squad{}.
% % 	They found human annotators achieved an Exact Match of $31.7\%$, significantly lower than the $82.3\%$ on the original, well-formed input, and much lower than the neural model could achieve.
% % 	(They also show that humans do not prefer \mppi{} queries over a random sub-sequence of words dervied from the original query, in order to predict the answer.)

% % 	We conducted the same annotation task for BERT and XLNet models on SQuAD to examine if significant pre-training, and superior performance affects the human interpretability of \mppi{}s.
% % 	The results are shown in Table~\ref{human-f1}.
% % 	We also provide the random baseline for comparison, comprising of randomly selected tokens from the query, to match the length distribution of BERT's \mppi{} queries.
	
% % 	\begin{table}[t]
% % 		\small
% % 		\centering
% % 		\begin{tabular}{lr}
% % 			& \textsc{Human F1 (EM)} \\
% % 			\toprule
% % 			\textsc{Original} &  91.2 (82.3) \\
% % 			\abr{DrQA$^\dagger$} & - (31.7) \\
% % 			\abr{BERT-B} &  41.6 (32.0) \\
% % 			\abr{XLNet-L} & 37.6 (26.0) \\
% % 			\midrule
% % 			\abr{BERT-B*} & 60.7 (43.5) \\
% % 			\midrule
% % 			\abr{Random} & 26.5 (17.0) \\
% % 			\bottomrule
% % 		\end{tabular}
% % 		\caption{\label{human-f1}
% % 			The mean human performance (in F1 and Exact Match) on different variants of \mppi{}s for \squad{}.
% % 			The mean was computed over $100$ examples. \\
% % 			$^\dagger$ Human performance cited from \citet{feng2018pathologies} \\
% % 			$^*$ Indicates the model was trained with \mppi{} regularization.
% % 		}
% % 	\end{table}
	
% % 	In Table~\ref{human-f1} we see the same behavior for \abr{BERT} and \abr{XLNet}.
% % 	Compared to the ``Original" human performance on \squad{}, their \mppi{}s are far worse for humans to make accurate predictions.
% % 	Instead, there appears to be no significant human interpretability difference between the \mppi{}s generated by large pre-trained models and those generated by non-pretrained models. 
% % 	Additionally, we observe human performance on these \mppi{}s are slightly better than ``Randomly" shortened queries, and \mppi{} regularization significantly improves interpretability.
	
% 	\section{Are \mppi{}s Invariant to Random Seed?}
	
% 	One of the preliminary questions in our investigation was whether changing the random training seed significantly altered the \mppi{} produced by a model.
% 	If it were the case that this had a drastic effect, we might suspect \mppi{}s were somewhat random, or the product of meangingless over-confidence on out-of-distribution inputs.
% 	Table~\ref{appendix-random-seed} illustrates the random seed experiment in full. 
% 	Training $10$ SQuAD models, each with different random seeds, we generate \mppi{}s on the $2k$ SQuAD evaluation set, and compare 5 pairs. 
% 	We measure the mean Generalized Jaccard Similarity of \mppi{}s produced by $2$ models trained with different seeds.
	
% 	We see the similarity between \mppi{}s trained with different seeds far exceed those of Rand-A, and Rand-B, which are akin to a ``random" simulation of \mppi{}s.
% 	As with our previous random baselines these are generated by randomly sampling tokens from the original query, preserving word order, and ensuring that the length distribution matches that of the actual \mppi{}s to which they are being compared.
	
% 	\begin{table}
% 		\centering
% 		\begin{tabular}{llr}
% 			\hline
% 			\textbf{Seed A} & \textbf{Seed B} & \textbf{JS / EM} \\
% 			\hline
% 			0 & 1 & 55.0 / 31.7 \\
% 			2 & 3 & 56.8 / 33.2 \\
% 			4 & 5 & 58.3 / 34.7 \\
% 			6 & 7 & 57.4 / 33.2 \\
% 			8 & 9 & 58.1 / 35.2 \\
% 			\hline
% 			{}  & Overall & 57.1 / 33.6 \\
% 			\hline
% 			Rand-A & Rand-B & 13.8 /  0.9 \\
% 			\hline
% 		\end{tabular}
% 		\caption{\label{appendix-random-seed}
% 			Observing the Jaccard Similarity and Exact Match between \mppi{}s on the SQuAD $2k$ evaluation set, we see significant token overlap despite seed differences. 
% 			In contrast, the randomly generated sequences, preserving the length distribution of \mppi{}s, produces far less similar token sequences.
% 		}
% 		\vspace*{-.4cm}
% 	\end{table}
	
% 	\section{Are \mppi{}s Invariant to Training Domain?}
	
% 	We discussed the invariance of \mppi{}s to training domain at length in the paper for BERT.
% 	For completeness, we provide the raw results for BERT in Table~\ref{bert_dataset-mppi-similarity} and for XLNet in Table~\ref{xlnet_dataset-mppi-similarity}.
% 	These results show that \mppi{}s are far more similar to one another, even when training domain is different.
% 	The random baseline, in parenthesis, once again  shows the Jaccard Similarity we would expect if \mppi{}s were purely random.
	
% 	\begin{table*}
% 		\resizebox{\linewidth}{!}{\begin{tabular}{lrrrrrr}
% 				{\textbf{Train Dataset}} & \multicolumn{6}{c}{\textbf{Reduction Dataset}} \\
% 				\hline{}
% 				{} & \abr{SQuAD} & \abr{HotPotQA} & \abr{NewsQA} & \abr{NatrualQ} & \abr{TriviaQA} & \abr{SearchQA} \\
% 				\hline{}
% 				\abr{SQuAD} & - (-) & 31.4 (8.8) & 41.0 (21.6) & 29.2 (12.5) & 24.9 (10.9) & 11.9 (9.6) \\
% 				\abr{HotPotQA} & 39.7 (12.8) & - (-) & 39.6 (18.8) & 33.8 (13.5) & 25.8 (10.7) & 16.6 (12.6) \\
% 				\abr{NewsQA} & 41.1 (13.0) & 31.6 (7.2) & - (-) & 35.2 (12.5) & 25.8 (10.8) & 13.3 (9.4) \\
% 				\abr{NatrualQ} & 37.5 (12.7) & 28.7 (7.1) & 40.2 (17.9) & - (-) & 25 (10.7) & 15.0 (11.0) \\
% 				\abr{TriviaQA} & 33.3 (13.0) & 27.7 (8.0) & 34.8 (18.1) & 29.2 (15.4) & - (-) & 23.1 (15.2) \\
% 				\abr{SearchQA} & 23.4 (12.3) & 16.8 (7.8) & 24.7 (17.2) & 24.4 (14.6) & 23.4 (11.9) & - (-) \\
% 				\hline
% 				{Average} & 35.0 (12.8) & 27.2 (7.5) & 36.1 (18.7) & 30.4 (13.7) & 25.0 (11.0) & 16.0 (11.6) \\
% 		\end{tabular}}
% 		\caption{\label{bert_dataset-mppi-similarity}
% 			The Jaccard Similarity (\%) between \abr{BERT} generated \mppi{}s, across domains. The Random baseline \mppi{}s are in parentheses.
% 		}
% 	\end{table*}
	
% 	\begin{table*}
% 		\resizebox{\linewidth}{!}{\begin{tabular}{lrrrrrr}
% 				{\textbf{Train Dataset}} & \multicolumn{6}{c}{\textbf{Reduction Dataset}} \\
% 				\hline{}
% 				{} & \abr{SQuAD} & \abr{HotPotQA} & \abr{NewsQA} & \abr{NatrualQ} & \abr{TriviaQA} & \abr{SearchQA} \\
% 				\hline{}
% 				\abr{SQuAD} & - (-) & 25.8 (9.0) & 37.7 (19.7) & 30.9 (11.1) & 18.1 (10.5) & 22.7 (26.3) \\
% 				\abr{HotPotQA} & 28.4 (15.3) & - (-) & 31.2 (17.6) & 31.5 (12.4) & 17.8 (12.0) & 27.1 (25.5) \\
% 				\abr{NewsQA} & 31.8 (13.1) & 25.3 (8.2) & - (-) & 36.6 (11.9) & 20.6 (9.0) & 13.3 (11.7) \\
% 				\abr{NatrualQ} & 29.9 (12.9) & 24.2 (8.4) & 40.2 (16.8) & - (-) & 22.3 (11.0) & 19.2 (16.3) \\
% 				\abr{TriviaQA} & 25.6 (14.8) & 19.0 (8.0) & 29.8 (17.4) & 29.2 (13.7) & - (-) & 31.2 (20.6) \\
% 				\abr{SearchQA} & 21.6 (13.8) & 15.5 (7.7) & 25.2 (15.1) & 24.6 (14.1) & 28.3 (13.4) & - (-) \\
% 				\hline
% 				{Average} & 27.5 (14.0) & 22.0 (8.3) & 32.8 (17.3) & 30.6 (12.6) & 21.4 (11.2) & 22.7 (20.1) \\
% 		\end{tabular}}
% 		\caption{\label{xlnet_dataset-mppi-similarity}
% 			The Jaccard Similarity (\%) between \abr{XLNet} generated \mppi{}s, across domains. The Random baseline \mppi{}s are in parentheses.
% 		}
% 	\end{table*}
	
% 	\section{Do QA Models Generalize to different \mppi{} Domains?}
	
% 	Expanding on the \mppi{} generalization analysis in Section 3.2, we provide the raw results.
% 	The cross-domain generalization of BERT and XLNet models on \mppi{}s sourced from different training domains is available in Table~\ref{appendix-raw-bbc-cross-domain-generalization} and Table~\ref{appendix-raw-xlc-cross-domain-generalization} respectively. Figure~\ref{fig:xlnet-cross-domain-f1} visualizes how well \abr{XLNet} generalizes to different \mppi{} domains.
% 	The results mirror those of \abr{BERT} shown in the main paper.

% 	\begin{figure}[h]
% 		\includegraphics[width=1\linewidth]{figures/xlnet-mppi-crossdomain.pdf}
% 		\caption{\abr{XlNet} performance with different training sets (y-axis), and evaluation sets (x-axis). Bars measure the F1 score on the $2k$ evaluation set, colored by input type.}
% 		\label{fig:xlnet-cross-domain-f1}
% 	  \end{figure}
	
% 	\begin{table*}
% 		\small
% 		% \addtolength{\tabcolsep}{-3pt}
% 		\centering
% 		\begin{tabular}{llrrrrrr}
% 			\hline
% 			\textbf{\begin{tabular}{@{}c@{}}Train \\ Dataset\end{tabular}} & \textbf{\begin{tabular}{@{}c@{}}Query \\ Type\end{tabular}} & \textbf{SQuAD} & \textbf{HotpotQA} &\textbf{NewsQA} & \textbf{NaturalQ} & \textbf{TriviaQA} & \textbf{SearchQA}\\
% 			\hline
% 			SQuAD & Original & 87.74 & 56.31 & 48.81 & 21.53 & 56.74 & 52.62 \\
% 			SQuAD & \mppi{} & 87.74 & 28.84 & 31.68 & 13.52 & 43.02 & 30.93 \\
% 			SQuAD & Random \mppi{} & 26.42 & 16.19 & 19.69 & 9.55 & 13.01 & 17.46 \\
% 			\hline
% 			TriviaQA & Original & 54.64 & 71.04 & 42.27 & 47.53 & 51.85 & 34.45 \\
% 			TriviaQA & \mppi{} & 34.25 & 71.04 & 24.67 & 32.28 & 33.85 & 18.91 \\
% 			TriviaQA & Random \mppi{} & 15.21 & 32.23 & 15.92 & 25.49 & 14.12 & 12.67 \\
% 			\hline
% 			NaturalQ & Original & 75.28 & 58.18 & 77.78 & 37.84 & 54.08 & 51.16 \\
% 			NaturalQ & \mppi{} & 55.15 & 40.43 & 77.78 & 24.32 & 44.52 & 34.25 \\
% 			NaturalQ & Random \mppi{} & 23.28 & 23.94 & 38.43 & 18.39 & 16.32 & 17.34 \\
% 			\hline
% 			SearchQA & Original & 40.25 & 59.44 & 32.58 & 78.11 & 35.93 & 20.61 \\
% 			SearchQA & \mppi{} & 24.84 & 41.67 & 21.24 & 78.11 & 24.96 & 15.9 \\
% 			SearchQA & Random \mppi{} & 11.92 & 24.69 & 14.73 & 45.7 & 12.34 & 9.7 \\
% 			\hline
% 			HotpotQA & Original & 71.52 & 53.4 & 52.51 & 38.9 & 75.09 & 47.03 \\
% 			HotpotQA & \mppi{} & 49.52 & 34.56 & 37.23 & 20.66 & 75.09 & 30.38 \\
% 			HotpotQA & Random \mppi{} & 21.09 & 19.28 & 24.92 & 15.2 & 17.76 & 17.88 \\
% 			\hline
% 			NewsQA & Original & 78.16 & 60.91 & 59.94 & 33.79 & 56.53 & 68.19 \\
% 			NewsQA & \mppi{} & 61.32 & 39.17 & 42.48 & 19.44 & 48.58 & 68.19 \\
% 			NewsQA & Random \mppi{} & 22.78 & 20.4 & 22.74 & 15.05 & 14.49 & 24.83 \\
% 			\hline
% 		\end{tabular}
% 		\caption{\label{appendix-raw-bbc-cross-domain-generalization}
% 			Cross-Domain Generalization of \abr{BERT} Base models on different types of inputs. Values correspond to F1 scores on the question answering $2k$ evaluation set specified by the column.
% 		}
% 	\end{table*}
	
	
% 	\begin{table*}
% 		\small
% 		% \addtolength{\tabcolsep}{-3pt}
% 		\centering
% 		\begin{tabular}{llrrrrrr}
% 			\hline
% 			\textbf{\begin{tabular}{@{}c@{}}Train \\ Dataset\end{tabular}} & \textbf{\begin{tabular}{@{}c@{}}Query \\ Type\end{tabular}} & \textbf{SQuAD} & \textbf{HotpotQA} &\textbf{NewsQA} & \textbf{NaturalQ} & \textbf{TriviaQA} & \textbf{SearchQA}\\
% 			\hline
% 			SQuAD & Original & 93.92 & 64.97 & 66.62 & 15.13 & 70.51 & 65.06 \\
% 			SQuAD & \mppi{} & 93.95 & 17.75 & 39.95 & 6.37 & 41.36 & 35.27 \\
% 			SQuAD & Random \mppi{} & 31.0 & 12.86 & 21.12 & 7.3 & 16.19 & 17.85 \\
% 			\hline
% 			TriviaQA & Original & 67.55 & 78.15 & 51.7 & 67.69 & 57.85 & 44.97 \\
% 			TriviaQA & \mppi{} & 31.77 & 78.18 & 27.8 & 43.63 & 32.34 & 22.24 \\
% 			TriviaQA & Random \mppi{} & 17.01 & 34.03 & 16.03 & 33.18 & 14.54 & 13.27 \\
% 			\hline
% 			NaturalQ & Original & 85.61 & 67.84 & 82.06 & 42.92 & 67.43 & 60.82 \\
% 			NaturalQ & \mppi{} & 63.02 & 35.73 & 82.06 & 20.44 & 46.19 & 42.95 \\
% 			NaturalQ & Random \mppi{} & 31.74 & 23.31 & 36.07 & 18.05 & 19.98 & 22.45 \\
% 			\hline
% 			SearchQA & Original & 55.25 & 74.37 & 45.43 & 84.08 & 45.33 & 32.82 \\
% 			SearchQA & \mppi{} & 25.6 & 47.5 & 26.33 & 84.08 & 29.41 & 18.57 \\
% 			SearchQA & Random \mppi{} & 15.92 & 33.29 & 16.81 & 53.58 & 15.57 & 12.13 \\
% 			\hline
% 			HotpotQA & Original & 82.85 & 61.03 & 61.93 & 23.98 & 80.28 & 54.19 \\
% 			HotpotQA & \mppi{} & 51.11 & 14.57 & 40.95 & 9.08 & 80.3 & 23.66 \\
% 			HotpotQA & Random \mppi{} & 27.83 & 14.0 & 23.89 & 14.03 & 21.33 & 15.25 \\
% 			\hline
% 			NewsQA & Original & 88.56 & 69.32 & 67.61 & 30.74 & 69.14 & 73.17 \\
% 			NewsQA & \mppi{} & 65.64 & 29.66 & 48.56 & 11.0 & 45.15 & 73.12 \\
% 			NewsQA & Random \mppi{} & 30.47 & 16.29 & 20.27 & 6.64 & 15.71 & 25.35 \\
% 			\hline
% 		\end{tabular}
% 		\caption{\label{appendix-raw-xlc-cross-domain-generalization}
% 			Cross-Domain Generalization of \abr{XLNet} Large models on different types of inputs. 
% 			Values correspond to F1 scores on the question answering $2k$ evaluation set specified by the column.
% 		}
% 	\end{table*}
%     \bibliography{anthology}
% 	\bibliographystyle{acl_natbib}
% 	\clearpage{}
% \end{document}
